# Supplementary material for: Ephemeral Antibubbles: Spatiotemporal Evolution from Direct Numerical Simulations
Source: arXiv:2103.16780 ancillary file (2021-03-31)
Supplement: Supplementary file 1 [file supplementary_30-March-21.pdf]

# Supplementary Material for Ephemeral Antibubbles: Spatiotemporal Evolution from Direct Numerical Simulations

Nairita Pal[a],[1] Rashmi Ramadugu[b],[2] Prasad Perlekar[c],[2] and Rahul Pandit[d3]

[1]Los Alamos National Laboratory, NM 87545, USA

[2]TIFR Center for Interdisciplinary Sciences, Tata Institute of Fundamental Research, Gopanpally, Hyderabad, 500046, India

[3]Center for Condensed Matter Theory, Department of Physics, Indian Institute of Science, Bangalore 560012, India.

(Dated: March 30, 2021)

In this Supplemental Material we present some details of the dynamics of the system of an antibubble rising under gravity, which we have discussed in the main paper.

## THICKNESS AT THE SOUTH POLE OF THE ANTIBUBBLE

In the main paper, we have described two methods for determining the antibubble-breakup time. We give details of the second method here.

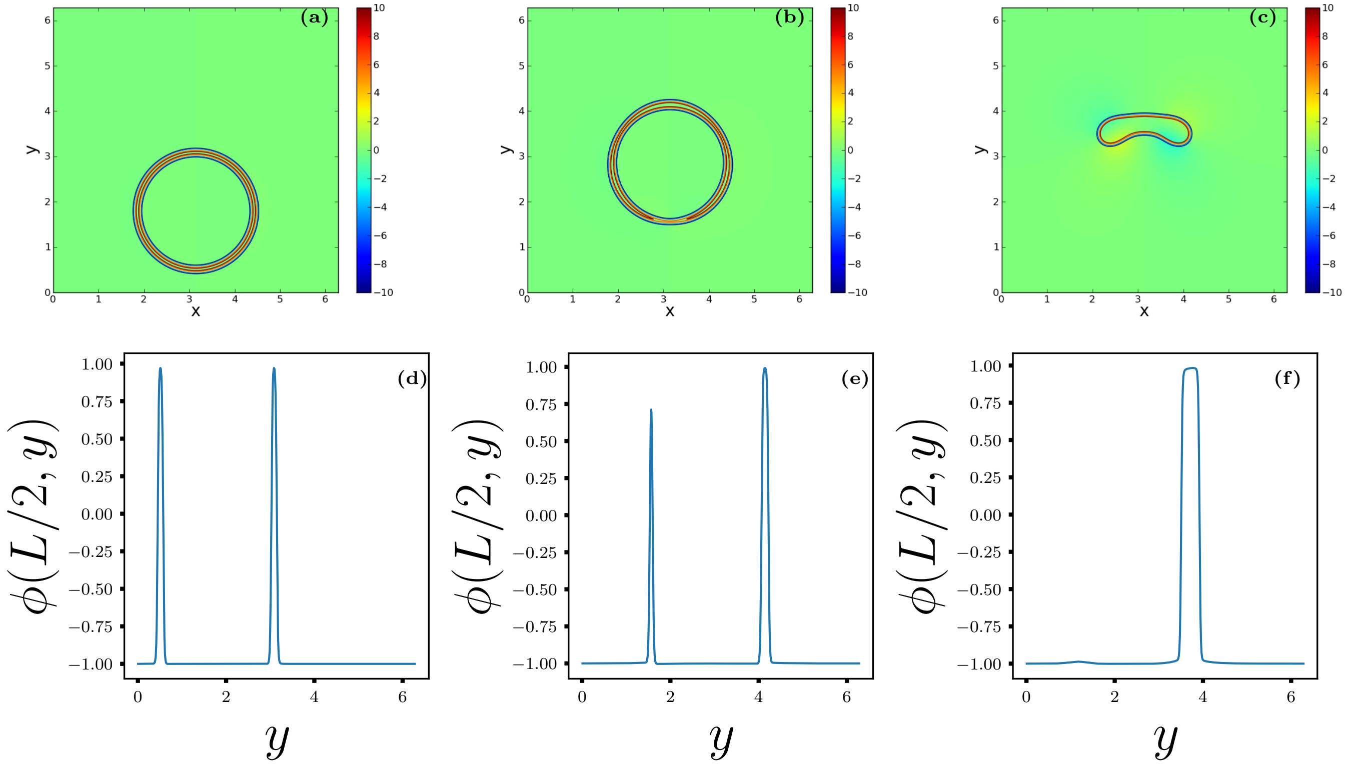


FIG. S1. Top row : Contours of the $\phi$ field superimposed on the pseudocolor plot of the vorticity field of the antibubble in 2D at (a) $t = 0$; (b) $t = 3.75\tau_g$, and (c) $t = 4.9\tau_g$. Bottom row: Plots of $\phi$ versus $y$ at $x = L/2$ at (d) $t = 0$ (initial snapshot); (e) $t = 3.75\tau_g$; and (f) $t = 4.9\tau_g$. This plot shows that we can track the thickness, $h_{min}$, at the South pole of the antibubble by tracking the width of the peak in the plots of $\phi(L/2, y)$, which corresponds to the South pole of the antibubble (i.e., $y < y_{cm}$, $y_{cm}$ being the $y$ coordinate of the center of mass of the antibubble. These plots are for DNS run R72 in Table II in the main paper.

[a]nairitap2009@gmail.com
[b]rashmi.ramadugu@gmail.com
[c]perlekar@tifrh.res.in
[d]rahul@physics.iisc.ernet.in; also at Jawaharlal Nehru Center For Advanced Scientific Research, Jakkur, Bangalore, India.

As the antibubble rises under gravity, its high-density core of the antibubble comes down, and the thickness at the South pole of the antibubble decreases with time. Eventually, the film ruptures at the South pole of the antibubble. at the time $\tau_2$. To find the thickness of the film $h_{min}$ at the South pole of the antibubble, we scan along the vertical $y$ axis at $x = N/2$. The film is the region in which $\phi > 0$. To find the thickness at the South pole of the antibubble, we scan over $y - y_{cm} < 0$, where $y_{cm}$ denotes the $y$ coordinate of the center-of-mass of the antibubble:

$$y_{cm} = \sum_{y \in \phi < 0} y\phi(x, y). \tag{S1}$$

We find the time $\tau_2$ of the collapse of the antibubble by noting the time at which $h_{min} = 0$.

The tracking of the thickness of the antibubble is easiest if we plot $\phi(L/2, y)$, i.e., the one-dimensional (1D) section of $\phi(x, y)$ at $x = L/2$ (see Fig. S1). This 1D profile of $\phi(L/2, y)$, at $t = 0$, is a superposition of two tangent-hyperbolic functions, with the two peaks separated by a distance $(R_0 + R_1)$. The distance between these two peaks, at any instant of time, gives the distance between the two poles of the antibubble. As time elapses, the peak at the South pole of the antibubble starts decreasing (see Fig. S1). Finally, at $t = \tau_2$, when collapse occurs, $\phi$ at the South pole attains the value it has in the majority phase; at this time there is only one peak at the North pole.

When the antibubble breaks, the surface tension energy is converted to kinetic energy of the antibubble. The rate of change of surface-tension energy is given by $\sigma d\mathcal{S}(t)/dt$, where $\mathcal{S}(t)$ is the outer perimeter of the antibubble; and the released kinetic energy is given by $E_M = \int_{S_f} \left(\rho v^2(\boldsymbol{x}, t)\right) d\boldsymbol{x}$, where $S_f$ is the area of the majority phase surrounding the minority phase, which causes the film to retract. Hence, $\sigma d\mathcal{S}(t)/dt \propto dE_M/dt$; we check this explicitly in our DNS: We calculate $\mathcal{S}(t)$ by finding the length of the $\phi = 0$ contour. We then calculate $d\mathcal{S}/dt$ numerically, by using a first-order finite-difference scheme. In Fig. S2(a) (blue curve) we plot $d\mathcal{S}/dt$ versus $t/\tau_g$. We then calculate the fluid-energy dissipation rate $\varepsilon(t) = \langle \nu |\omega(\boldsymbol{x}, t)|^2 \rangle_{\boldsymbol{x}}$, where $\langle\rangle_{\boldsymbol{x}}$ denotes the average over space, and $\omega = \nabla \times \boldsymbol{u}$ is the fluid vorticity, along the perimeter $\mathcal{S}(t)$ of the antibubble. We see that the plot of $d\mathcal{S}/dt$ versus $t/\tau_g$, in Fig. S2(a), almost overlaps with that of $\varepsilon(t)$ versus $t/\tau_g$ in Fig. S2(a); note that $\sigma$ is constant along the perimeter. In Figs. S2(b)-(f) we show the perimeter of the antibubble as it retracts.

## EFFECT OF THE KINEMATIC VISCOSITY EFFECTS

In Fig. S3, we plot $\tau_1$ versus $Bo$ for different values of $Sc$. From this plot, we note that, with the increase in $Sc$; a log-log plot $\tau_1/\tau_g$ versus $Sc$ is given in the main paper.

## FINAL STATE OF A STATIC ANTIBUBBLE

An antibubble is an inherently unstable structure, even in the absence of gravity. If it is allowed to evolve for a long time, with no background flow or gravity, diffusion dominates: after a long period of time, the inner circular disc of the antibubble diffuses out, and we are left with a droplet of the minority phase, instead of an annular ring, inside the majority phase (see Fig. S4). Oscillations appear in the kinetic-energy time series $E(t)$; these decrease with time as we show in Fig. S5, where the blue (green) curve shows $E(t)$ for an antibubble with $R_0/h_0 = 8$, $(R_0/h_0 = 9)$. The lower the sizeof an antibubble, the lower its perimeter and, therefore, the lower the fluid kinetic energy that is generated because of the diffusion of the minority phase into the majority phase. The important point to note is that the time scale, over which the antibubble becomes a droplet, is very large compared to time scale of the rupture of an antibubble under gravity. We have seen, in the main paper, that the timescale of gravity-induced antibubble rupture is $\tau_g = \sqrt{R_0/Ag} = 1.16$; by contrast, for an antibubble of the same size, the diffusion timescale is $\tau = R_0^2/D = 240$, which is about 243 times slower.

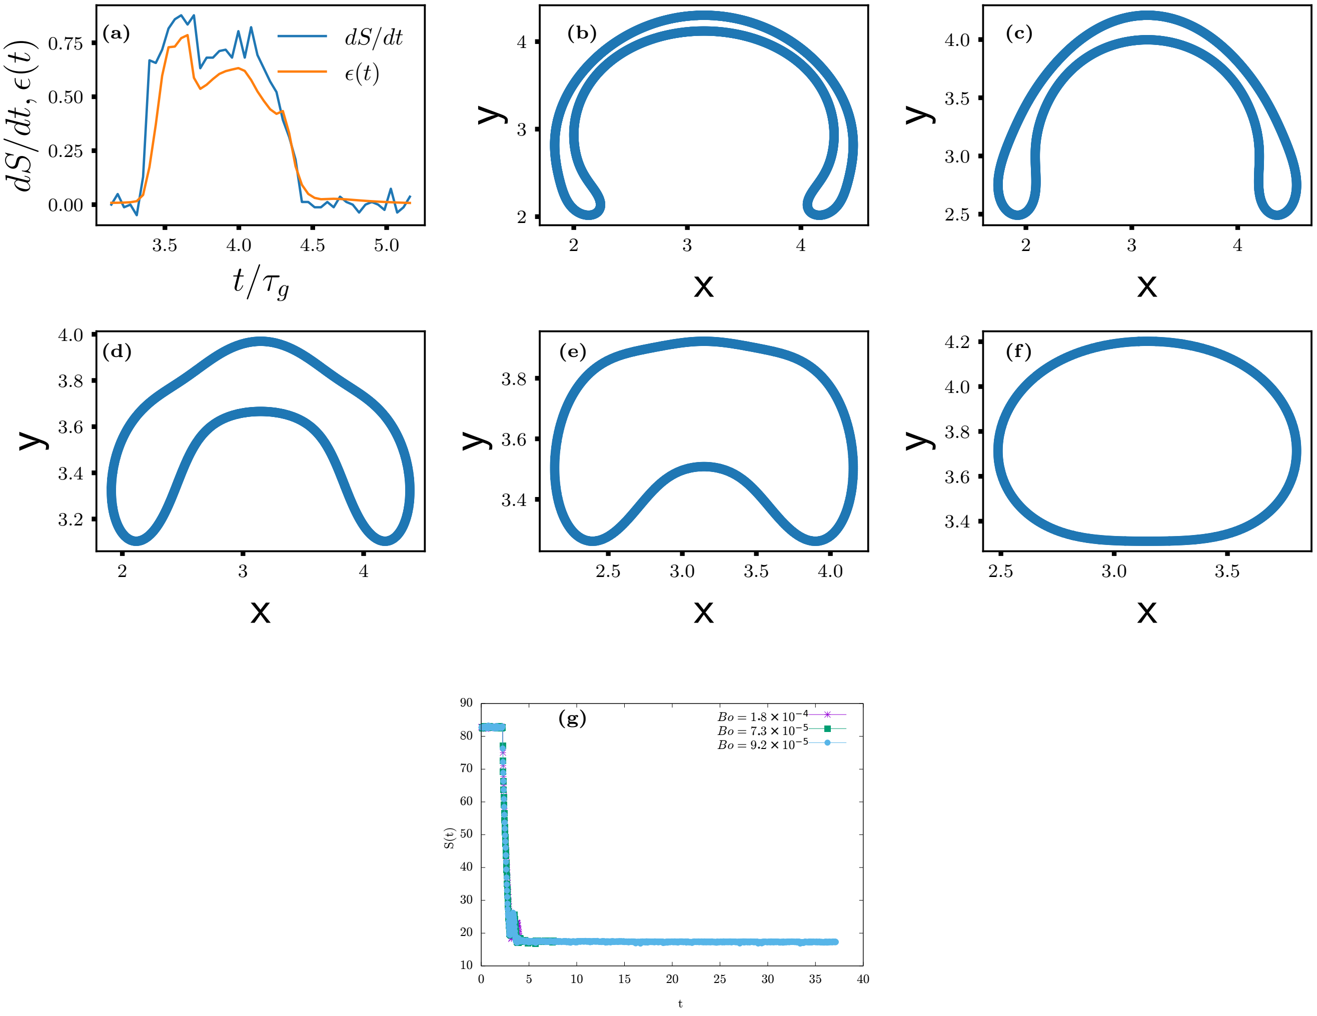


FIG. S2. (a) Plot versus $t/\tau_g$ of $d\mathcal{S}(t)/dt$ (blue line) and $dE_M/dt$ (green line). Plot of the perimeter of the droplet at (b) $t = 4.25\tau_g$; (c) $t = 4.45\tau_g$; (d) $t = 4.75\tau_g$; (e) $t = 4.9\tau_g$; (f) $t = 5.15\tau_g$; (g) plots of $d\mathcal{S}/dt$ vand $\varepsilon(t)$ versus $t/\tau_g$; (g) evolution of the antibubble surface with time. These plots are from DNS run `R72` in Table II in the main paper.

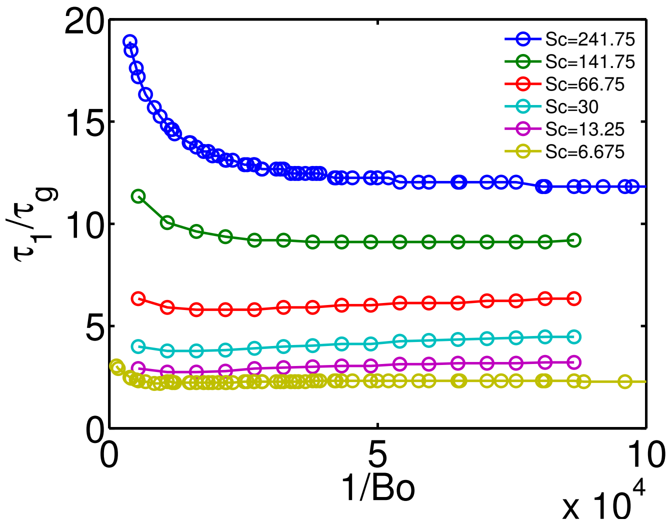


FIG. S3. Plot of $\tau_1/\tau_g$ versus $1/Bo$, for $Sc = 241.75$ (blue line with circles, DNS run R1, $Sc = 141.75 = 0.567$ (green line with circles), $Sc = 66.75$ (red line with circles), $Sc = 30$ (light blue line with circles), $Sc = 13.25$ (magenta line with circles), $Sc = 6.675$ (yellow line with circles). These plots show how the lifetime of an antibubble varies with $Sc$.

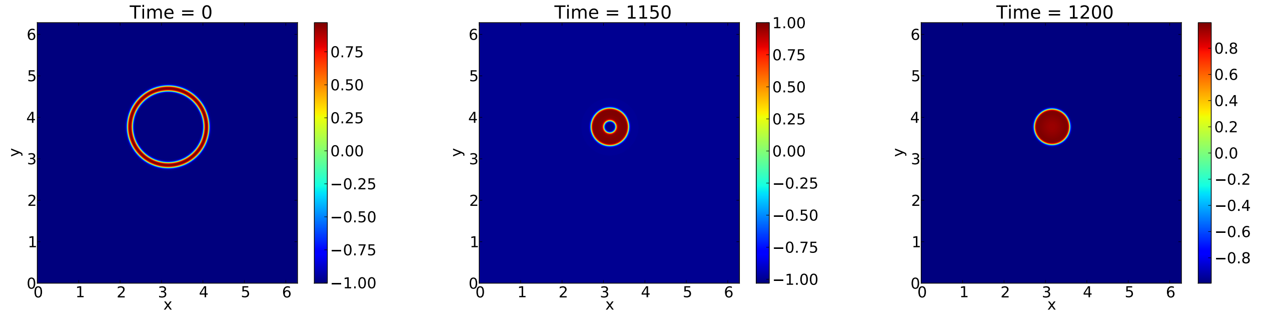


FIG. S4. Pseudocolor plots of the $\phi$ field with antibubble radius $R_0/h_0 = 7$, $\nu = 0.967$ and $\sigma = 3.31$ (i.e, $Bo = 9.11 \times 10^{-5}$ ), at (a) $t = 0$; (b) $t = 1150$; and (c) $t = 1200$. All times are given in units of $2500\delta t$.

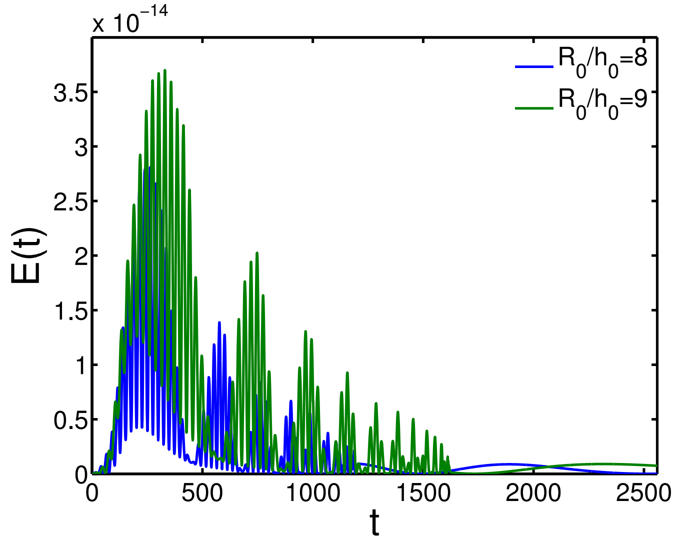


FIG. S5. Plots of kinetic energy $E(t)$ versus $t$ for static (a) antibubble with $R_0/h_0 = 8$ (blue line), and (b) antibubble with $R_0/h_0 = 9$ (green line).

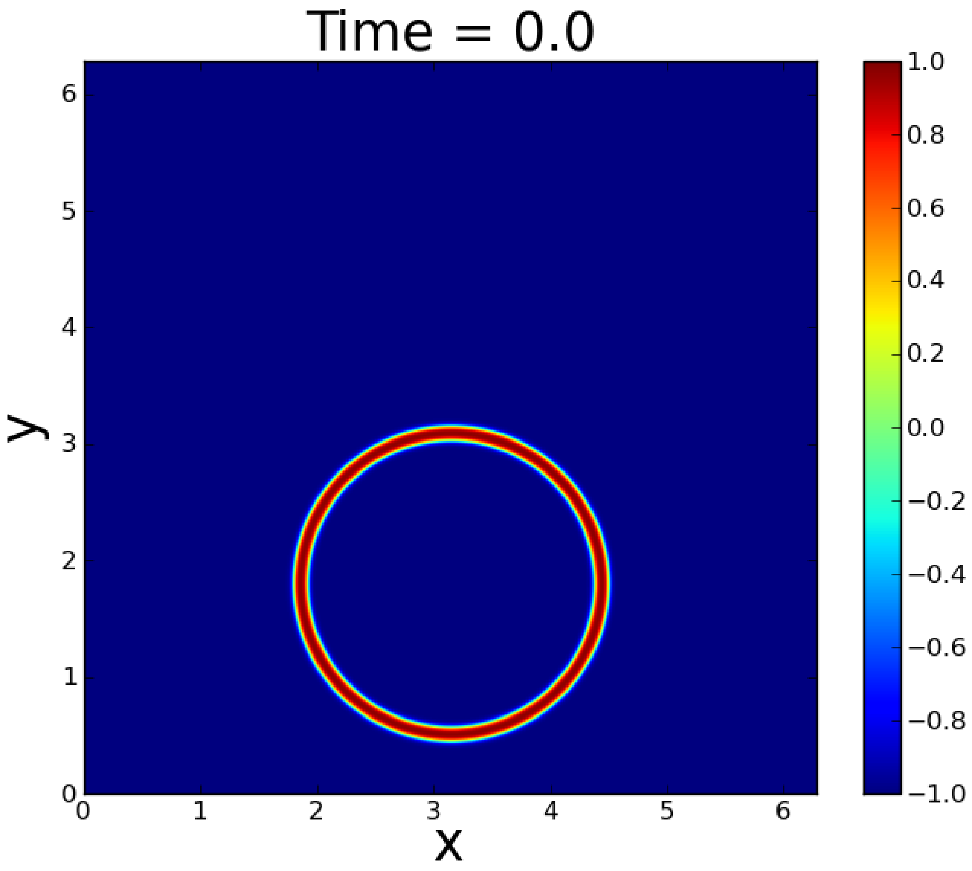


FIG. S6. Supplementary Video 1 : Pseudocolor plots of the CHNS $\phi$ field with antibubble radius $R_0/h_0 = 7$, for $\nu = 0.007$ and $\sigma = 16.6$ (i.e, $Bo = 0.01$, from our 2D DNS run `R16`) (see I in the main paper). Time is in units of $\tau_g$.

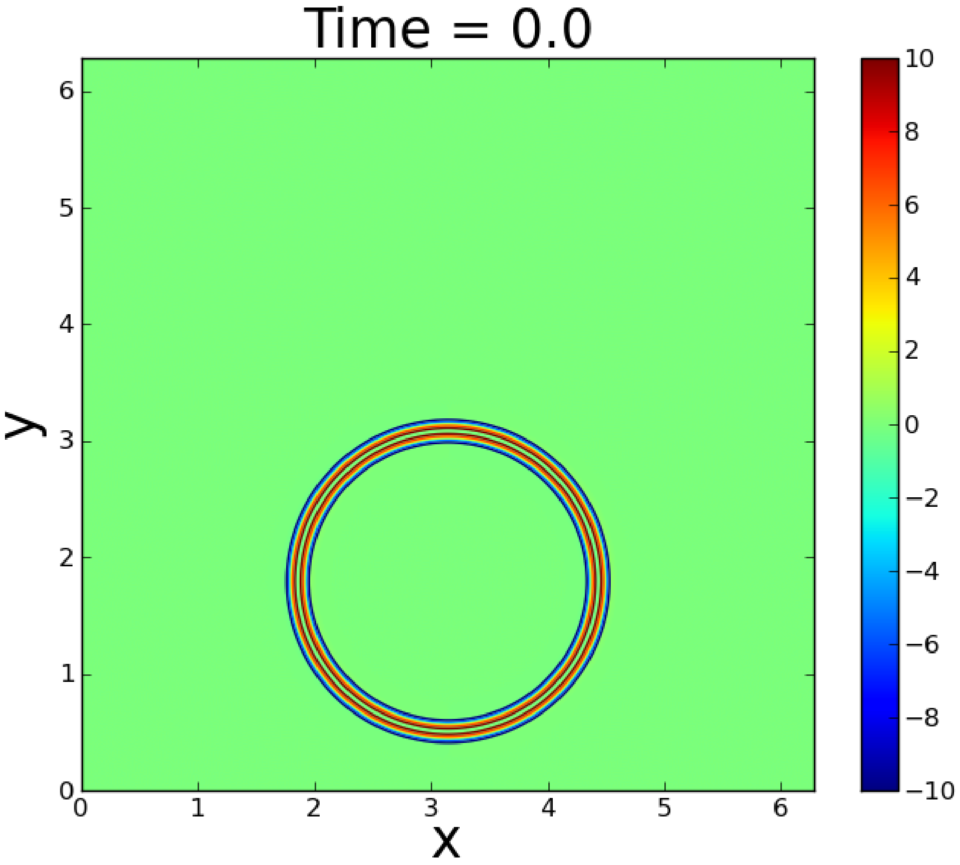


FIG. S7. Supplementary Video 2 : Pseudocolor plots of the CHNS $\omega$ field with antibubble radius $R_0/h_0 = 7$, for $\nu = 0.007$ and $\sigma = 16.6$ (i.e, $Bo = 0.01$, from our 2D DNS run `R16`) (see I in the main paper). Time is in units of $\tau_g$.
